# Supplementary material for: Effective Magnetic Switching of THz Signal in Planar Structured Spintronic Emitters
Source: arXiv:2407.21623 source file (2024-11-01)
Supplement: Supplementary file 1 [file Supplementary.pdf]

# Supplementary Information: Effective Magnetic Switching of THz Signal in Planar Structured Spintronic Emitters

## I. SUPPLEMENTARY NOTE I: Y-COMPONENT THZ RADIATION POLARIZATION

The ZnTe detector is sensitive to the X and Y components of the THz radiation polarization. Similarly to how the Longitudinal Kerr Effect is sensitive to the X component of magnetization, due to the magnetization being parallel to the plane of incident light, the Transverse Kerr Effect is sensitive to the Y component of magnetization, as the magnetization is perpendicular to the plane of incident light. Transitioning from detecting one component to another is achieved by rotating the ZnTe detector by 90 degrees, which allows us to detect either the X or Y component of the THz radiation.

Such measurements allow us to gain insights into the remagnetization process. The corresponding hysteresis loops for the THz generators with periods $T = 1000\,\mu\text{m}$, $50\,\mu\text{m}$, and $8\,\mu\text{m}$ for stripes grown perpendicular to the easy axis are shown in Figure 1. The hysteresis loops for stripes grown parallel to the easy axis, with periods $T = 300\,\mu\text{m}$, $100\,\mu\text{m}$, $8\,\mu\text{m}$, and $4\,\mu\text{m}$, are depicted in Figure 2. The difference between the two series of samples (with the easy axis of magnetization induced by a magnetic field applied during sample growth along or perpendicular to the microstripes) is even more pronounced. For samples with the induced easy axis perpendicular to the stripes (Figures 1(a, b)), we achieve almost sharp switching of linear THz polarization during remagnetization in this direction. It can also be noted that for samples with a wide stripe (1000 µm; Figure 1(a)), remagnetization proceeds through a multidomain state, whereas for narrow stripes (50 µm and 8 µm; Figure 1(b, c)), the domain formation process is suppressed.

For the magnetic field applied along the easy axis (along the stripes, Figure 2), we observe a relatively small Y-component of the THz signal (an order of magnitude smaller than the X-component), as expected. However, it can be quite large compared to the signal for the other direction of the applied magnetic field, demonstrating the suppression of the domain formation process and almost sharp switching, as mentioned above.

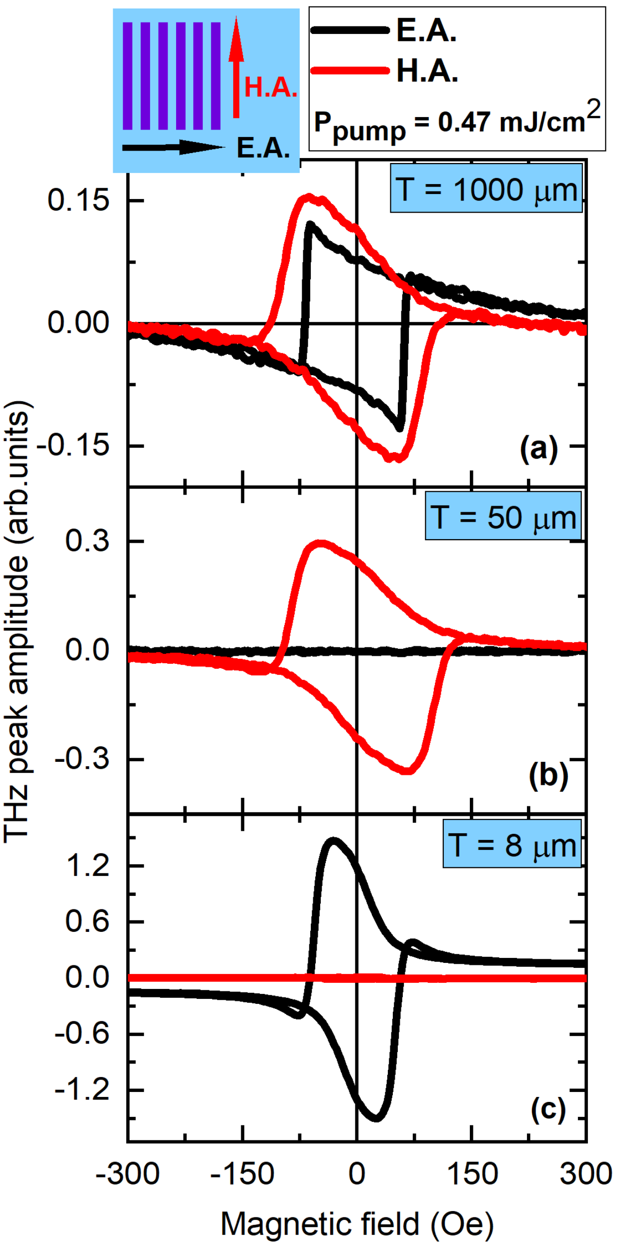


FIG. 1: Hysteresis loop for y-polarization (oriented along the applied magnetic field) of THz signal for the magnetic field along or perpendicular to the easy axis for (a) 1000 µm, (b) 50 µm grating period and E.A. perpendicular to stripes. The orientation of easy and hard axis are shown in the insets.

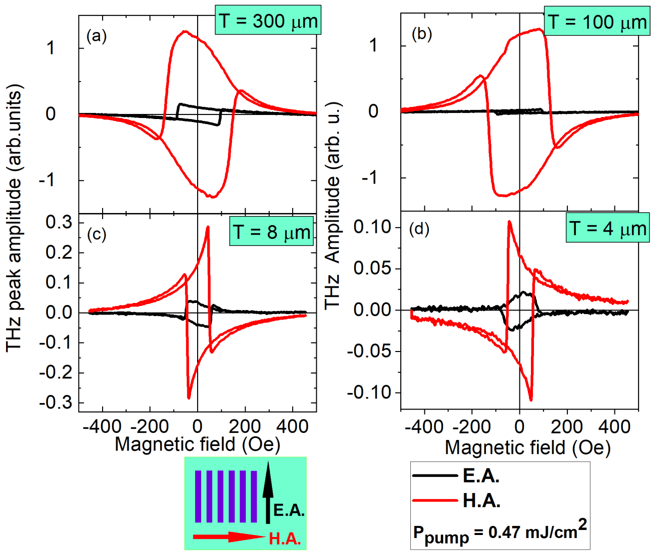


FIG. 2: Hysteresis loop for y-polarization (oriented along the applied magnetic field) of THz signal for the magnetic field along or (a) 300 µm, (b) 100 µm, (c) 8 µm, (d) 4 µm grating period and E.A. parallel to stripes. The orientation of easy and hard axis are shown in the insets.

## II. SUPPLEMENTARY NOTE II

Figure 3 shows the angular diagrams of the THz signal measured for the Ex component of the THz field with the WGP rotated by an angle $\varphi_2$ in a magnetic field of 2 kOe. In the position of the WGP corresponding to $\varphi_2 = 0$, the Ex component of the THz field completely passes through the polarizer. The measurements were performed for two configurations of samples relative to the applied magnetic field: with magnetization along E.A. (black curve) and along H.A. (red curve). Both series of samples with different directions of magnetic anisotropy were also considered: structures with E.A. directed along the stripes (the upper row of structures with a period of $T = 300, 100, 8,$ and $2\,\mu$m) and structures with E.A. directed perpendicular to the stripes (the lower row of structures with a period of $T = 1000, 500, 50,$ and $8\,\mu$m). The measured peak-to-peak amplitude of the THz signal is determined in accordance with the expression:

$$\Delta S(t) = f(\varphi_2, E_{\mathrm{THz}}(\varphi_1)) \times \cos(\theta(t)),$$

where $\theta$ is the phase difference between $\Delta S(t)$ and the reference signal, $t$ is the delay time, and $f(\varphi_2, E_{\mathrm{THz}}(\varphi_1))$ is a function describing the dependence of the electric field of the THz wave on the rotation angle of the WGP polarizer plane $\varphi_2$ and the angle $\varphi_1$ between the polarization of the THz wave and the [110] axis of the ZnTe crystal [1, 2]. All parameters obtained from the fitting ($E_{\mathrm{THz}}$ – amplitude of the THz field in arbitrary units, $e$ – coefficient of ellipticity and $\varphi_1$ angle for both E.A. and H.A. axis) are presented in Table I.

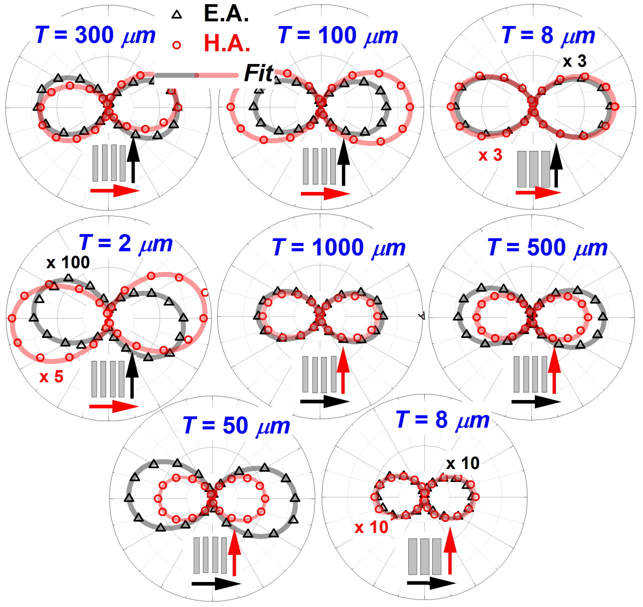


FIG. 3: THz amplitude angular diagrams measured during WGP rotation for structures with E.A. directed along (T = 300, 100, 8, and 2 µm) and perpendicular to the stripes (1000, 500, 50, and 8 µm). The magnetic field was applied along the E.A. axis (black curve) and along the H.A. (red curve).

| $T, \mu$m | E.A. direction | $E_{\mathrm{THz}}$, arb.un. | e | $\varphi_1$, deg (E.A.) | $\varphi_1$, deg (H.A.) |
|---|---|---|---|---|---|
| 1000 | perpendicular to stripes | $0.54 \pm 0.05$ | $0.72 \pm 0.06$ | $3.4 \pm 1.5$ | $3.2 \pm 1.7$ |
| 500 | perpendicular to stripes | $0.54 \pm 0.04$ | $0.74 \pm 0.05$ | $4.8 \pm 1.4$ | $-0.6 \pm 1.7$ |
| 50 | perpendicular to stripes | $0.64 \pm 0.03$ | $0.67 \pm 0.04$ | $12.7 \pm 1.5$ | $-3.3 \pm 1.7$ |
| 8 | perpendicular to stripes | $0.65 \pm 0.06$ | $0.7 \pm 0.1$ | $4 \pm 3$ | $3 \pm 3$ |
| 300 | along stripes | $0.70 \pm 0.02$ | $0.55 \pm 0.03$ | $3.9 \pm 1.2$ | $-29 \pm 2$ |
| 100 | along stripes | $0.55 \pm 0.03$ | $0.74 \pm 0.04$ | $-2 \pm 3$ | $-2 \pm 3$ |
| 8 | along stripes | $0.51 \pm 0.05$ | $0.65 \pm 0.06$ | $2.9 \pm 1.2$ | $1.7 \pm 1.1$ |
| 4 | along stripes | $0.67 \pm 0.12$ | $0.65 \pm 0.11$ | $39 \pm 6$ | $-21 \pm 3$ |

TABLE I: Table of measurements and parameters.

## III. SUPPLEMENTARY NOTE III: THEORETICAL MODEL

This section contains a detailed description of the simple theoretical model that we use to fit the experimental data. We consider two different cases: the sample is magnetized perpendicular to the stripes (THz emission is effective) or along them (THz emission is suppressed).

For the Co/Pt sample magnetized perpendicularly to the stripes, the electric current provided by ISHE flows along the stripes, in accordance with the law $I \sim \theta_{SH} [\boldsymbol{n} \times \boldsymbol{M}]$, where $\boldsymbol{n}$ is the normal to the surface (direction of spin current flow), $\boldsymbol{M}$ is the magnetization of Co (direction of spin), $\theta_{SH}$ is the spin Hall angle governed by spin-orbit interaction in Pt. We neglect the charge accumulation at the ends of stripes supposing that they are very long ($l >> w$, where $l$ is the stripe length, $w$ its width). We also do not take into account the inductance in our simple model. Another supposition is that the power injected into a unit square of the emitter from magnetic system $p_i$ is constant irrespectively of the magnetization direction. This is correct in the case of ideal spin sink (we neglect spin accumulation in Pt). Then power injected into one stripe is determined as $P_i = p_i lw$. The stripe resistance in this case is $R_{||} = \rho l/hw$, where $\rho$ is resistivity, $h$ is the thickness of the stripe, which gives the power dissipated by alternating electric current at one stripe equal to $I_{||}^2 \rho l/2hw$. Then magnitude of alternating electric current flowing through one stripe is

$$I_{||} \sim \sqrt{\frac{2p_i w^2 h}{\rho}}. \tag{1}$$

In order to find the THz emission rate, we need to calculate the average electric current density (taking into account the 1/2 filling factor):

$$\langle j_{||} \rangle = \frac{1}{2}\frac{I_{||}}{wh} \sim \sqrt{\frac{p_i}{2\rho h}}. \tag{2}$$

Then the amplitude of THz field is proportional to this current density multiplied by the volume of the emitter.

If the sample is magnetized along the stripes we take into account charge accumulation caused by the ISHE current which flows perpendicular to the stripes. In order to determine the current in this case we ought to calculate the high-frequency conductance taking into account active resistance determined by film conductivity and reactance mainly determined by electrical capacitance of the system. The resistance is $R_{||} = \rho w/hl$, and the power dissipated at the active resistance per one stripe is $P_R = I_\perp^2 \rho w/2hl$, similar to the previous case. Then we roughly estimate the power accumulated at the stripe edges by supposing that the charge is conducted at very thin wires with the diameter equal to the layer thickness $d = h$. The electric potential created by one such wire is $\varphi(\boldsymbol{r}) \sim qLog\left(\frac{r}{d/2}\right)$, where $q = \pm I_\perp / i\omega$ depending on the stripe side, $\omega$ is the frequency of electric current $I_\perp$. We then calculate the energy power accumulated at such a charged edge (which is supposed to be far away from the grating edge) in the electric field created by all other stripes' edges (the number of stripes is determined as $N = L/2w >> 1$, where $L$ is the characteristic grating width):

$$P_c = (1+\xi)\frac{I_\perp^2}{2l\omega} Log\left(\frac{L}{w}\right). \tag{3}$$

The constant $\xi$ appears here due to the screening of electric field by metallic stripes (one half of the charged wires is screened for each wire, while the other is not). However it is close to $\xi \approx 1$ if the stripe thickness is much smaller than their width ($h << w$) which is obviously satisfied in our structures. Taking into account that total power injected into one stripe is $P_i = p_i lw = P_R + P_c$ it is then straightforward to find the electric current per one stripe:

$$I_\perp \sim \sqrt{\frac{2p_i l^2 h}{\rho + \frac{2}{\omega}\frac{h}{w} Log\left(\frac{L}{w}\right)}}. \tag{4}$$

Once again, in order to find the THz emission rate, we need to calculate the average electric current density (taking into account the 1/2 filling factor and that the geometry of current flow is different from previous case described in (2)):

$$\langle j_\perp \rangle = \frac{1}{2}\frac{I_\perp}{lh} \sim \sqrt{\frac{p_i}{2h\left(\rho + \frac{2}{\omega}\frac{h}{w} Log\left(\frac{L}{w}\right)\right)}}. \tag{5}$$

Then the amplitude of THz field is proportional to this current density multiplied by the volume of the emitter which is the same as in previous case. The ratio of THz signal emitted in two considered cases is then

$$Ratio = \frac{\langle j_{||} \rangle}{\langle j_\perp \rangle} = \sqrt{1 + \frac{h}{L}\frac{2}{\rho\omega}\frac{L}{w} Log\left(\frac{L}{w}\right)}. \tag{6}$$


[1] F. Zainullin, D. Khusyainov, M. Kozintseva, and A. Buryakov, Polarization analysis of thz radiation using a wire grid polarizer and znte crystal, Russian Technological Journal **10**, 74 (2022).

[2] A. Buryakov, A. Gorbatova, P. Avdeev, E. Lebedeva, K. Brekhov, A. Ovchinnikov, N. Gusev, E. Karashtin, M. Sapozhnikov, E. Mishina, *et al.*, Efficient co/pt thz spintronic emitter with tunable polarization, Applied Physics Letters **123** (2023).
